# Supplementary material for: Flexoelectricity in soft elastomers and the molecular mechanisms underpinning the design and emergence of giant flexoelectricity
Source: arXiv:2105.12291 ancillary file (2021-05-26)
Supplement: Supplementary file 1 [file Flexoelectricity_in_soft_elastomers-PNAS-SI--Grasinger,_Mozaffari,_and_Sharma.pdf]

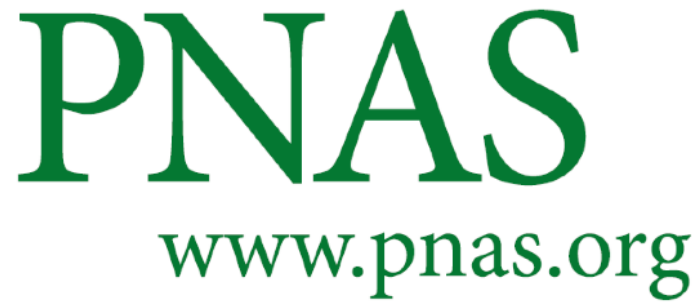

## **Supplementary Information for**

### **Flexoelectricity in soft elastomers and the molecular mechanisms underpinning the design and emergence of giant flexoelectricity**

**Matthew Grasinger, Kosar Mozaffari and Pradeep Sharma**

**Pradeep Sharma**  
**E-mail: [psharma@uh.edu](mailto:psharma@uh.edu)**

#### **This PDF file includes:**

Supplementary text  
Figs. S1 to S4 (not allowed for Brief Reports)  
SI References

## Supporting Information Text

### 1. The effect of dipole-dipole interactions

In the main article, we neglected dipole-dipole interactions in order to make an approximate statistical mechanics treatment of the electroelasticity of freely-jointed and wormlike polymer chains with polar monomers. Neglecting dipole-dipole interactions results in a good approximation when the energy of dipole-dipole interactions is small relative to the thermal energy of the chain,  $nkT$ . In this section, we use numerical simulation to understand more precisely what conditions must be satisfied for dipole-dipole interactions to be negligible, as well as to verify that the analytical results are indeed accurate when these conditions are met. Surprisingly, the simulations also suggest something stronger: that the stretch–polarization relationship—obtained analytically in the main article—is valid even when dipole-dipole interactions are non-negligible.

We use the Markov chain Monte Carlo (MCMC) method for numerical simulation\* (see (1), for example). For convenience, we simulate the chain in the fixed force ensemble, as opposed to the fixed end-to-end vector ensemble†; and take advantage of the fact that, in the “thermodynamic limit”, the two ensembles are equivalent in the sense that their respective free energies are related by the proper Legendre transform. The Hamiltonian used in the MCMC simulations, including dipole-dipole interactions, is given by:

$$\mathcal{H}_{\text{MCMC}} = \sum_{i=1}^n (-\boldsymbol{\mu}_i \cdot \mathbf{E}) - \left( b \sum_{i=1}^n \hat{\mathbf{n}}_i \right) \cdot \mathbf{F} - \sum_{i=1}^n \sum_{j=i+1}^n \frac{3(\boldsymbol{\mu}_i \cdot \hat{\mathbf{z}}_{ij})(\boldsymbol{\mu}_j \cdot \hat{\mathbf{z}}_{ij}) - \boldsymbol{\mu}_i \cdot \boldsymbol{\mu}_j}{4\pi\epsilon_0 z_{ij}^3} \quad [1]$$

where,  $\mathbf{z}_{ij} = \mathbf{x}_i - \mathbf{x}_j$ ,  $\hat{\mathbf{z}}_{ij} = \mathbf{z}_{ij}/|\mathbf{z}_{ij}|$ ,

$$\mathbf{x}_k = \mathbf{x}_{k-1} + \frac{b}{2} \hat{\mathbf{n}}_k = b \sum_{i=1}^{k-1} \hat{\mathbf{n}}_i + \frac{b}{2} \hat{\mathbf{n}}_k; k = 1, 2, \dots, n; \mathbf{x}_0 = \mathbf{0}$$

are the monomer positions, and  $\mathbf{F}$  is the applied force on the chain; further, recall:  $\mathbf{E}$  is an applied electric field (i.e. electric field that would result if there were no dipoles present) and  $\boldsymbol{\mu}_i = \mathbf{M}_i \hat{\mathbf{n}}_i$ . In the simulations presented herein,  $\mathbf{M}$  is the same for every monomer in the chain, i.e.  $\mathbf{M}_i = \mathbf{M}$ ,  $i = 1, 2, \dots, n$ ; and, because of its simplicity and physical relevance, we choose  $\mathbf{M} = \mu \mathbf{I}$  for our examples where  $\mathbf{I}$  is the identity tensor. The first term in Eq. (1) is the energy of interaction between the monomer dipoles and the applied electric field, the second term is the work performed by the externally applied force on the chain, and the last term corresponds to the dipole-dipole interactions.

In the main article, we argue that dipole-dipole interactions are negligible when  $\tilde{\mu}^2 \ll 1$  where  $\tilde{\mu} := \mu/\sqrt{\epsilon_0 b^3 kT}$ . We assume this condition is met and, neglecting the interactions, we derive the free energy of the freely jointed chain with polar monomers. In this regime, the (normalized) tension in the chain that results from enforcing the end-to-end vector constraint is  $\boldsymbol{\tau} = \mathcal{L}^{-1}(\gamma) \hat{\mathbf{r}} - \beta \mathbf{M}^T \mathbf{E}$  where  $\mathcal{L}^{-1}$  is the inverse Langevin function,  $\gamma := r/nb$  is the chain stretch,  $\hat{\mathbf{r}}$  is the direction of the end-to-end vector, and  $\beta = 1/kT$ . In the thermodynamic limit, we can relate this to the applied force in the fixed force ensemble,  $\boldsymbol{\tau} = \mathbf{F}b/kT$ . This result is compared with the MCMC simulations with zero applied field, (i.e.  $\mathbf{E} = 0$ ),  $n = 100$ , and  $\tilde{\mu} = 0.1, 0.25, 0.5$ , and  $1.0$  in Fig. S1. One can see that the agreement is nearly exact when  $\tilde{\mu} = 0.1$  and  $\tilde{\mu} = 0.25$ . The chain elasticity seems to vary, however, when  $\tilde{\mu} \geq 0.5$ . This suggests that when  $\tilde{\mu} \leq 0.25$  dipole-dipole interactions are indeed negligible.

Next we consider the relationship between the chain stretch and its polarization (i.e. its net dipole) since this is what is most relevant to the flexoelectric effect in elastomers. We obtain this relationship for the freely jointed chain (in the fixed end-to-end vector ensemble) by taking a partial derivative of the free energy:  $\mathbf{p} = -\partial \mathcal{F}/\partial \mathbf{E} = n\gamma \mathbf{M} \hat{\mathbf{r}}$ . This result is compared with the MCMC simulations in Fig. S2 where the normalized polarization,  $\tilde{p} := p/n\sqrt{\epsilon_0 b^3 kT}$ , is plotted as a function of chain stretch,  $\gamma$ , for  $\tilde{\mu} = 0.1, 1.0, 5.0$ , and  $10.0$ . (Here  $p = |\mathbf{p}|$  and, since  $\mathbf{M} = \mu \mathbf{I}$ , the chain polarization is in the  $\hat{\mathbf{r}}$  direction.) Remarkably, there is near perfect agreement, even in the cases where dipole-dipole interactions are clearly non-negligible (i.e.  $\tilde{\mu} = 1.0, 5.0$ , and  $10.0$ ). This suggests that the stretch–polarization relationship obtained analytically is valid even when dipole-dipole interactions are significant. Therefore, although one should expect the elasticity of the bulk elastomer to vary when transitioning from the regime where dipole-dipole interactions are negligible (i.e.  $\tilde{\mu} \leq 0.25$ ) to the regime where dipole-dipole interactions are significant (i.e.  $\tilde{\mu} > 0.5$ ), Fig. S2 suggests that its flexoelectricity will remain constant.

A natural way to probe the generality of Fig. S2 is to consider the effects of an applied electric field. Let the nondimensional electric field be given by  $\tilde{E} = E\mu/kT = E\tilde{\mu}\sqrt{\epsilon_0 b^3 kT}$ . Then Fig. S3 shows the stretch–polarization relationship for  $\tilde{E} = 1.0$  and  $\tilde{\mu} = 0.1, 1.0, 5.0$ , and  $10.0$  where the chain is being stretched in the direction of the electric field. Similarly, in Fig. S4, the stretch–polarization relationship is again shown but for the case where  $\mathbf{E} \cdot \mathbf{F} = 0$ ; that is, where the applied force on the chain is orthogonal to the electric field. Note that, in this case, the polarization is not necessarily in the direction of the applied electric field or force. It is, however, in the  $\hat{\mathbf{r}}$  direction, as expected. In either case, we see that, again, the analytical results show nearly exact agreement with the MCMC simulations—even when dipole-dipole interactions are significant. These results support the notion that the theory of flexoelectricity developed in the main article is quite general.

Before closing this section, we elucidate the physical reasons for why the stretch–polarization relationship appears to follow  $\mathbf{p} = n\gamma \mathbf{M} \hat{\mathbf{r}}$  regardless of the electric field or whether or not dipole-dipole interactions are significant. The stretch–polarization

\* The code used in this work can be found at <https://github.com/grasingerm/polymer-stats>.

† Sampling in the fixed end-to-end vector ensemble presents many difficulties. For one, generating a single trial move requires solving a nonlinear system of equations which scales with the number of monomers in the chain.

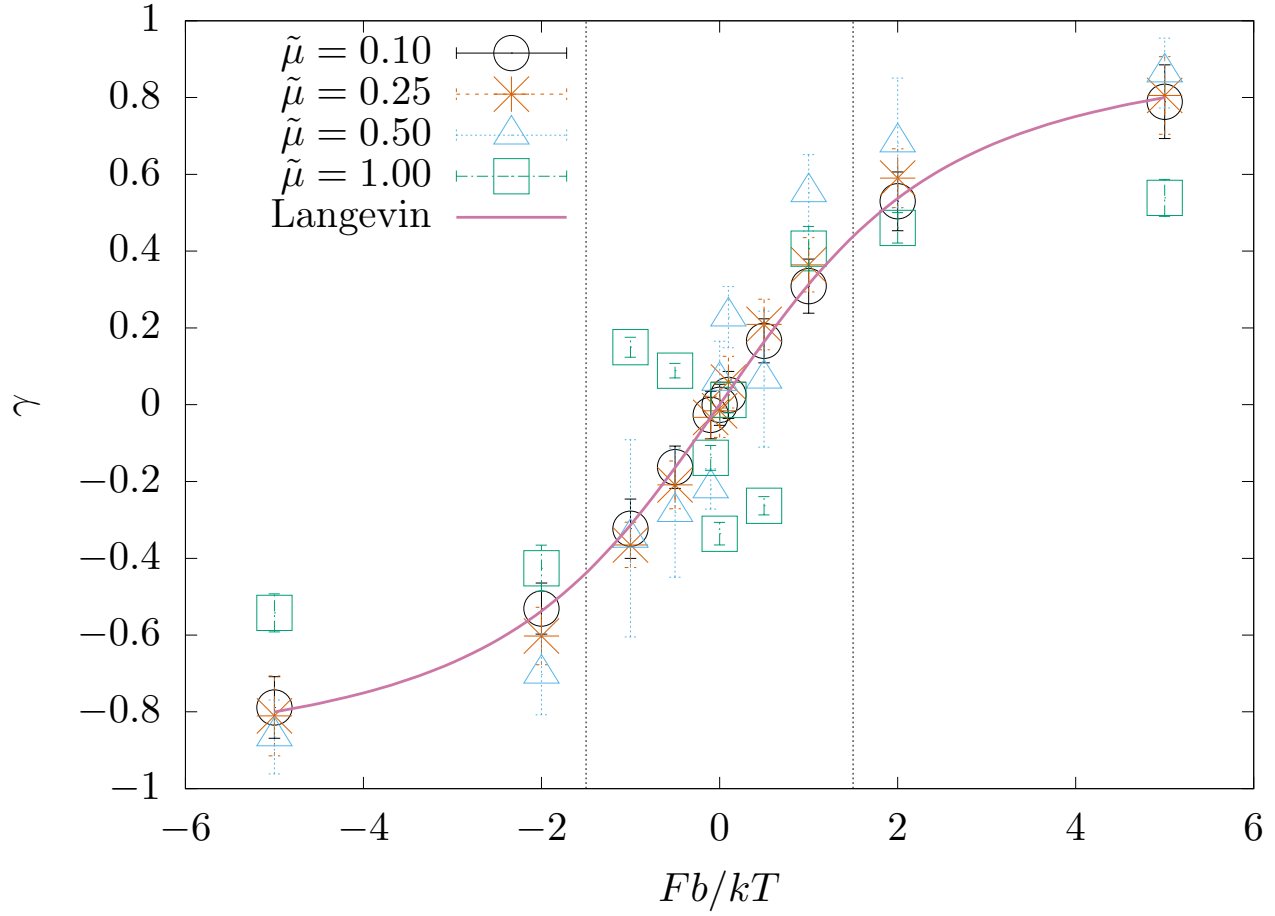

**Fig. S1.** MCMC simulations of the force-stretch relationship for a freely jointed chain with  $n = 100$ , dipole-dipole interactions, and  $\tilde{\mu} = \mu / \sqrt{\epsilon_0 b^3 kT} = 0.1, 0.25, 0.5$ , and  $1.0$ . When  $\tilde{\mu} \leq 0.25$  dipole-dipole interactions are negligible and the force-stretch relationship follows the Langevin function. When  $\tilde{\mu} \geq 0.5$  dipole-dipole interactions become significant and the chain elasticity is no longer described by the Langevin function. The error bars correspond to fluctuations in the chain stretch, i.e.  $\sqrt{\langle \gamma^2 \rangle - \langle \gamma \rangle^2}$ .

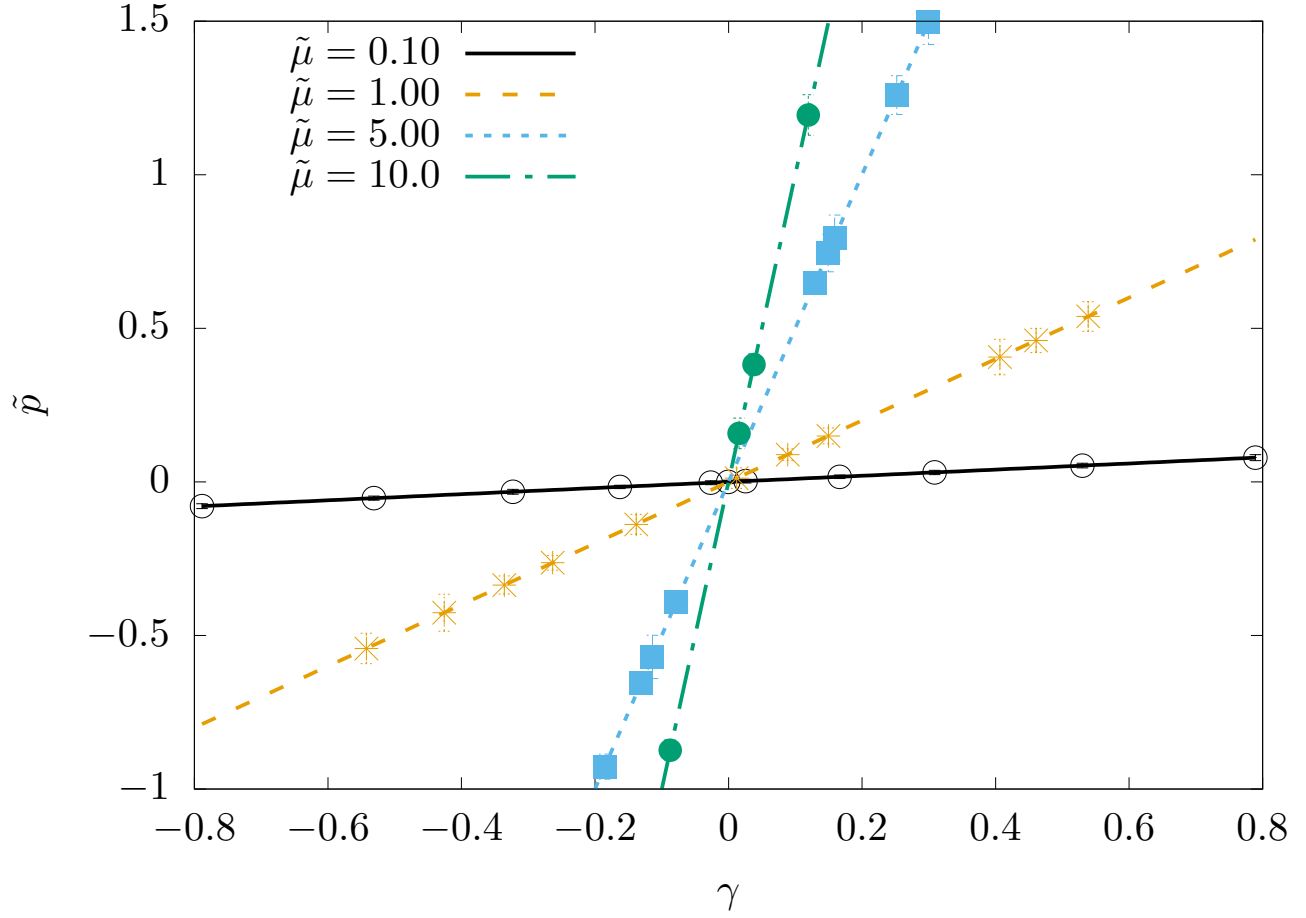

**Fig. S2.** MCMC simulations of the stretch-polarization relationship for a freely jointed chain with  $n = 100$ , dipole-dipole interactions, and  $\tilde{\mu} = \mu / \sqrt{\epsilon_0 b^3 kT} = 0.1, 1.0, 5.0$ , and 10.0. Here,  $\tilde{p} := p / n \sqrt{\epsilon_0 b^3 kT}$ , and the applied electric field is taken to be  $E = 0$ . The MCMC simulations agree nearly exactly with the analytical result  $\mathbf{p} = n\gamma \mathbf{M} \hat{\mathbf{r}}$ , even when dipole-dipole interactions are significant (i.e.  $\tilde{\mu} \geq 0.5$ ).

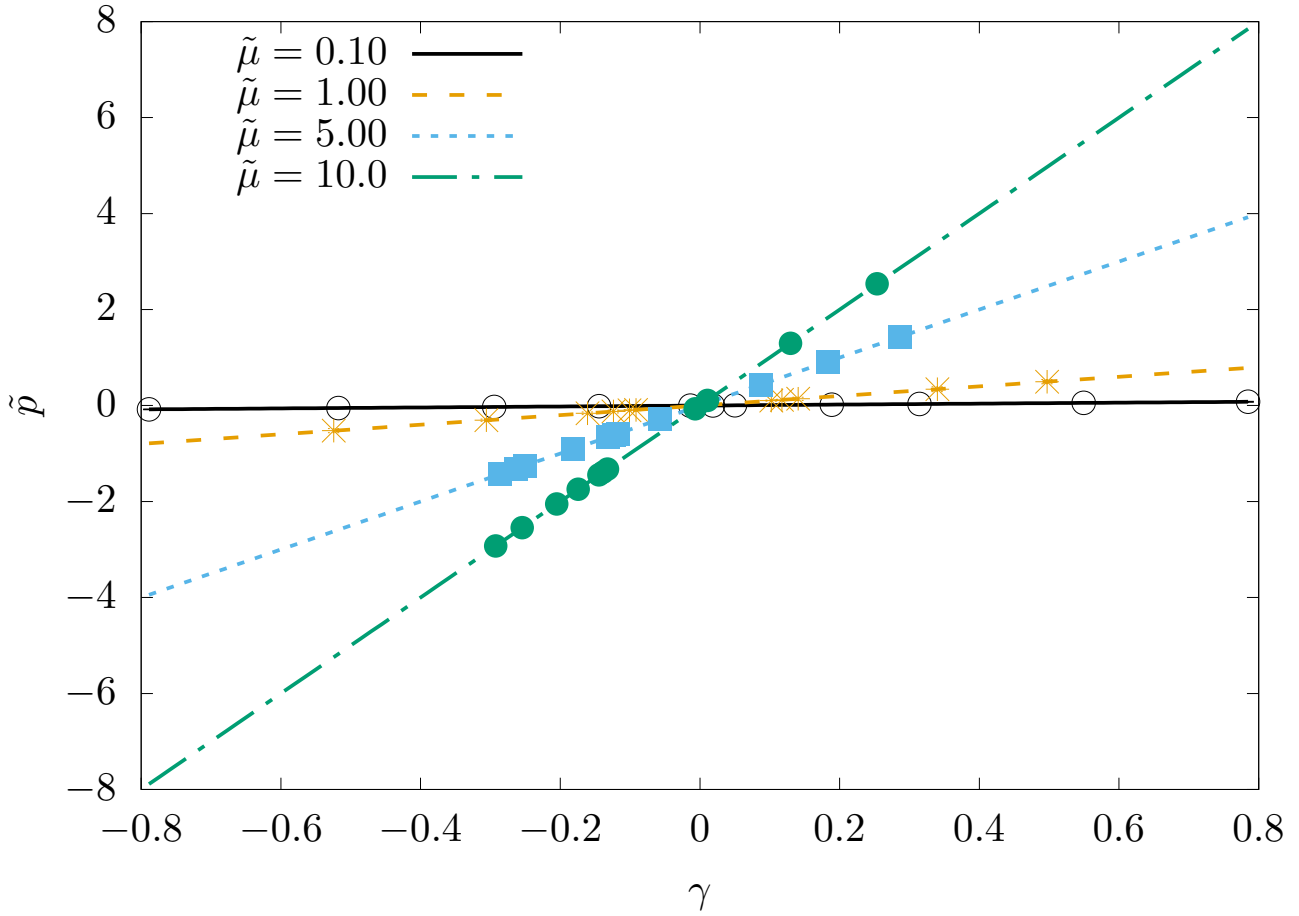

**Fig. S3.** MCMC simulations of the stretch–polarization relationship for a freely jointed chain with  $n = 100$ , dipole-dipole interactions, and  $\tilde{\mu} = \mu / \sqrt{\epsilon_0 b^3 kT} = 0.1, 1.0, 5.0$ , and  $10.0$ . Here the applied electric field is taken to be  $\tilde{E} = E\tilde{\mu} \sqrt{\epsilon_0 b^3 / kT} = 1.0$  and is in the direction of the applied force. Again, the MCMC simulations agree nearly exactly with the analytical result  $\mathbf{p} = n\gamma M \hat{\mathbf{r}}$ , even when dipole-dipole interactions are significant (i.e.  $\tilde{\mu} \geq 0.5$ ).

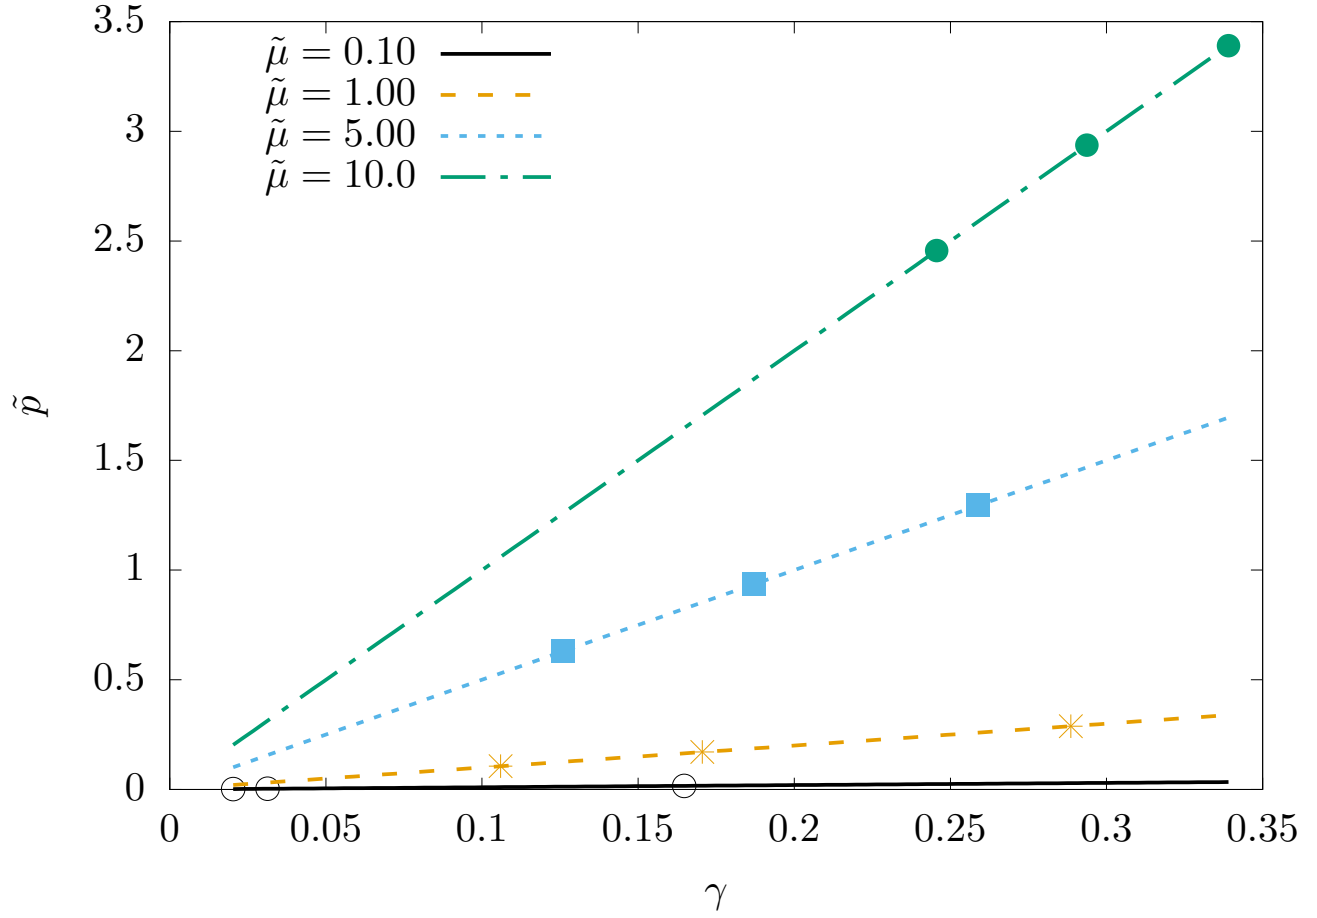

**Fig. S4.** MCMC simulations of the stretch–polarization relationship for a freely jointed chain with  $n = 100$ , dipole-dipole interactions, and  $\tilde{\mu} = \mu / \sqrt{\epsilon_0 b^3 kT} = 0.1, 1.0, 5.0$ , and  $10.0$ . Here the applied electric field is taken to be  $\tilde{E} = E \tilde{\mu} \sqrt{\epsilon_0 b^3 / kT} = 1.0$  and is such that  $\mathbf{E} \cdot \mathbf{F} = 0$ . Again, the MCMC simulations agree nearly exactly with the analytical result  $\mathbf{p} = n \gamma \mathbf{M} \hat{\mathbf{r}}$ , even when dipole-dipole interactions are significant (i.e.  $\tilde{\mu} \geq 0.5$ ).

relationship is clearly influenced by geometry, as expected, since we assume  $\boldsymbol{\mu}_i = M\hat{\mathbf{n}}_i$  and the end-to-end vector,  $\mathbf{r}$ , is directly related to the monomer directions,  $\hat{\mathbf{n}}_i, i = 1, 2, \dots, n$ . Another consequence of this assumed monomer dipole constitutive response is that the magnitude of the monomer dipoles do not vary with the local electric field; and therefore, neither an applied electric nor dipole-dipole interactions can affect the magnitude of dipoles along the chain. We are left then to consider the directions of the dipoles. In the main article, we explain why the density of monomers in a particular direction,  $\rho(\hat{\mathbf{n}})$ , is invariant with respect to the applied electric field. What we can say about the influence of dipole-dipole interactions is likely not as strong; instead, we expect  $\rho(\hat{\mathbf{n}})$  to depend on the significance of the dipole-dipole interactions. However, while this leads to a change in the chain elasticity (see Fig. S1, for example), it does not change the stretch–polarization relationship. This is because while an increasing significance of dipole-dipole interactions should lead to greater correlations between monomer directions and a collective-type of behavior should emerge, the influence of dipole-dipole interactions is isotropic. We should not expect a change in the average monomer direction and, hence, the average dipole direction. Making further use of this language and the correspondence between averaging and thermodynamic state variables, we see that the stretch–polarization relationship takes such a simple form almost by definition:

$$\mathbf{r} = b \left\langle \sum_{i=1}^n \hat{\mathbf{n}}_i \right\rangle,$$

$$\mathbf{p} = \left\langle \sum_{i=1}^n \boldsymbol{\mu}_i \right\rangle = M \left\langle \sum_{i=1}^n \hat{\mathbf{n}}_i \right\rangle = M \frac{\mathbf{r}}{b},$$

whereby  $\langle \square \rangle$  we mean the ensemble average of  $\square$ . So while pairwise correlations,  $\langle \hat{\mathbf{n}}_i \hat{\mathbf{n}}_j \rangle$ , for  $i = 1, 2, \dots, n, j = 1, 2, \dots, n$ , depend on the significance of dipole-dipole interactions, the chain polarization does not, which agrees with Fig. S2–S4.

## 2. Accounting for normalization constraint by variational approximation method

We aim to account for the normalization constraints of the monomers. Rewriting the normalization constraint from Eq. (12)<sub>2</sub> we have:

$$h(s) = \hat{\mathbf{n}}_i \cdot \hat{\mathbf{n}}_i - 1 \simeq \hat{\mathbf{n}}(s) \cdot \hat{\mathbf{n}}(s) - 1 = 0. \quad [2]$$

Here, we make a slight modification to this constraint and rewrite it in a weak form along the chain as follows:

$$h[\hat{\mathbf{n}}] = \sum_{i=1}^n \hat{\mathbf{n}} \cdot \hat{\mathbf{n}} - n = 0. \quad [3]$$

Incorporating the constraints using the Fourier representation of the Dirac delta we obtain the effective Hamiltonian as:

$$\mathcal{H}^{\text{eff}} \simeq \int_0^L \left( \frac{K}{2} \left| \frac{d\hat{\mathbf{n}}}{ds} \right|^2 - \frac{1}{b} \boldsymbol{\mathcal{E}} \cdot \hat{\mathbf{n}} - \frac{i}{L\beta} \mathbf{k} \cdot \hat{\mathbf{n}} - \frac{i\gamma}{L\beta} \hat{\mathbf{n}} \cdot \hat{\mathbf{n}} \right) ds + \frac{i}{L\beta} \mathbf{k} \cdot \mathbf{r} + \frac{i}{\beta} \gamma. \quad [4]$$

By definitions Eq. (15) and Eq. (16), we rewrite the effective Hamiltonian in equation Eq. (4) in Fourier space as:

$$\mathcal{H}^{\text{eff}} = L \sum_{q \in \mathbb{K}} \left( \frac{K}{2} q^2 |\omega(q)|^2 - \frac{i}{L\beta} \gamma |\omega(q)|^2 \right) - \frac{L}{b} \boldsymbol{\mathcal{E}} \cdot \omega(0) - \frac{i}{\beta} \mathbf{k} \cdot \omega(0) + \frac{i}{L\beta} \mathbf{k} \cdot \mathbf{r} + \frac{i}{\beta} \gamma, \quad [5]$$

As we mentioned earlier, handling this partition function in closed form is impractical due to the contribution of higher order terms from the normalization constraint. However, employing the variational approach, we can get a good estimation of the energy of the system. This approach is based on the Gibbs-Bogoliubov inequality which asserts that an upper bound to the free energy of the system can be obtained by(2):

$$\mathcal{F} \leq \mathcal{F}_{\text{var}} := \mathcal{F}_0 + \langle \mathcal{H} - \mathcal{H}_0 \rangle_0, \quad [6]$$

where  $\mathcal{F}_0$  is the free energy of the reference system with Hamiltonian  $\mathcal{H}_0$  and  $\langle \square \rangle_0$  is the statistical average of  $\square$  with respect to the defined reference system. This method is widely used for obtaining the free energy associated with the anharmonic Hamiltonians which has no exact solution. Accordingly, the effective Hamiltonian can be decomposed to:

$$\mathcal{H}^{\text{eff}} = \mathcal{H}_h + \mathcal{V}_h - \mathcal{V}_h + \mathcal{H}_{\text{anh}}, \quad [7]$$

where we did add and subtract the variational harmonic potential  $\mathcal{V}_h$  which has no consequence on the Hamiltonian but is the key to improve the upper bound. Generally, the upper bound can be improved if minimized with respect to the variational

parameter. Here, we define reference Hamiltonian  $\mathcal{H}_0$  as the harmonic part of the Hamiltonian plus an extra unknown variational potential, i.e  $\mathcal{H}_0 = \mathcal{H}_h + \mathcal{V}_h$ . The variational potential  $\mathcal{V}_h$  is defined as:

$$\mathcal{V}_h = \Upsilon/\beta \sum_{|q| \in \mathbb{K}} i\gamma(\omega_1(q) + \omega_2(q) + \omega_3(q)), \quad [8]$$

where the unknown coefficient  $\Upsilon$  accounts for the correlations between modes of deformation ( $\omega(q)$ ) and normalization mode ( $\gamma$ ). Introducing  $\alpha(q, k, \gamma) = [\omega_1(q_{min} : q_{max}), \omega_2(q_{min} : q_{max}), \omega_3(q_{min} : q_{max}), k_1, k_2, k_3, \gamma]$  where  $Size(\alpha) := m + 1$ , we rewrite  $\mathcal{H}_0$  as a quadratic function with the linear term as

$$\beta\mathcal{H}_0 = \sum_{i,j=1}^{m+1} \frac{1}{2} \alpha_i A_{ij} \alpha_j + b_i \alpha_i, \quad [9]$$

where  $\mathbf{A}$  and  $\mathbf{b}$  can be achieved from Eq. (5) by straight forward calculation and due to the addition of the variational potential. The free energy of the reference system  $\mathcal{F}_0$  with Hamiltonian  $\mathcal{H}_0$  can be obtained analytically since the reference Hamiltonian is harmonic. Hence, the variational free energy is given by:

$$\begin{aligned} \mathcal{F}_{var} &= \mathcal{F}_0 + \langle \mathcal{H} - \mathcal{H}_0 \rangle_0 = \mathcal{F}_0 + \langle \mathcal{H}_{anh} - \mathcal{V}_h \rangle_0 \\ &= \mathcal{F}_0 - i/\beta \left\langle \sum_{|q| \in \mathbb{K}} (\Upsilon\gamma(\omega_1(q) + \omega_2(q) + \omega_3(q)) + \gamma|\omega(q)|^2) \right\rangle_0, \end{aligned} \quad [10]$$

The correlations with respect to the reference Hamiltonian  $\mathcal{H}_0$  can be obtained by characteristics of generalized form of Gaussian integrals(3) as follows:

$$\begin{aligned} \langle \alpha_i \alpha_j \alpha_k \rangle_0 &= \Gamma_{ij} u_k + \Gamma_{ik} u_j + \Gamma_{jk} u_i + u_i u_j u_k \\ \langle \alpha_i \alpha_j \rangle_0 &= \Gamma_{ij} + u_i u_j, \end{aligned} \quad [11]$$

where  $\mathbf{\Gamma} = \mathbf{A}^{-1}$  and  $\mathbf{u} = -\mathbf{A}^{-1} \mathbf{b}$  and  $\mathbf{A}$  and  $\mathbf{b}$  are obtained from Eq. (9).

The calculation of  $\mathcal{F}_{var}$  is not straight forward for infinite number of the modes. Thus performing calculation on truncated number of modes gives us an estimation on the variational energy  $\mathcal{F}_{var}$  and thus the effect of normalization constraint on the polarization of the system. The minimum free energy is obtained by minimization with respect to the variational parameter  $\Upsilon$ , i.e.

$$\frac{\partial \mathcal{F}_{var}}{\partial \Upsilon} = 0. \quad [12]$$

Adopting this differentiation for free energy of truncated number of modes, is equivalent to minimizing the sensitivity of the free energy with respect to the variational parameter  $\Upsilon$ . Since we are ultimately interested in obtaining the effect of the normalization constraint on the polarization of the system, we take  $\mathbf{p} = -\frac{\partial \mathcal{F}}{\partial \mathbf{E}}$  and immediately observe that while this constraint affects the free energy of the system, it has no effect on the polarization of finite number of modes. Therefore, we take the polarization same as Eq. (20).

## References

1. Werner Krauth. *Statistical mechanics: algorithms and computations*, volume 13. Oxford University Press, 2006.
2. Samuel Safran. *Statistical thermodynamics of surfaces, interfaces, and membranes*. CRC Press, 2018.
3. Henk TC Stoof, Koos B Gubbels, and Dennis BM Dickerscheid. *Ultracold quantum fields*, volume 1. Springer, 2009.
